# Supplementary material for: Epidemic spread: limiting contacts to regular circles is not necessarily the safest option
Source: arXiv:2507.10257 ancillary file (2026-09-26)
Supplement: Supplementary file 1 [file SM.pdf]

# SUPLEMENTARY MATERIAL of article: Epidemic Spread: Limiting Contacts to Regular Circles Is Not Necessarily the Safest Option.

João Gabriel Simões Delboni[a], Gabriel Fabricius[a,b]

[a] *Instituto de Investigaciones Fisicoquímicas Teóricas y Aplicadas (INIFTA), CONICET and Facultad de Ciencias Exactas, Universidad Nacional de La Plata, CC 16, Suc. 4, 1900 La Plata, Argentina*

[b] *CCT CONICET La Plata, Consejo Nacional de Investigaciones Científicas y Técnicas, Argentina*

*Preprint submitted to Elsevier* *July 9, 2025*

## S1. Social Structure

In our stochastic SIR individual-based model, the structure is designed to provide a representative approximation of social interactions across different types of locations. Rather than attempting to replicate every nuance of real-world contact patterns—which would result in an overwhelming number of parameters—our approach is conceived as a compromise: it captures the essential heterogeneities of human interactions while avoiding the complexities that arise from overly detailed or high-dimensional models. Each individual is first assigned an age according to a predetermined age distribution that evenly allocates agents in 5-year intervals up to 75 years. This age assignment is used solely to guide subsequent processes, such as forming family households, assigning individuals to schools or workplaces, and linking them to additional social locations.

To incorporate distance-dependent effects for certain interactions (e.g., in schools or retail stores), the spatial environment is represented as a two-dimensional grid of size 300 by 300, where each cell corresponds to a unique household location. The grid is further subdivided into four equally sized regions ($Q$), representing broader geographic divisions of the city. Individuals within each region may occasionally interact with one another. These interactions rarely involve the same individuals and may represent chance encounters in large markets, on the street, in parks, public transportation, transport stations, or leisure venues, among others.

Individuals aged 20 or younger are assumed to live with their parents in family households consisting of four members, with generational age gaps between parents and children ranging from 21 to 39 years, selected to reflect observed data [1, 2]. For example, if a child is between 1 and 10 years old, their parents are assumed to be between 31 and 40; if the child is between 11 and 20, the parents are assumed to be between 41 and 50. For individuals aged 21–30, three types of household ($H$) configurations are allowed—pairs, single occupancy, and groups of four—with respective frequencies of 50%, 40%, and 10%. Likewise, for individuals aged 51–75, 34% are assumed to live in pairs, while the remaining individuals live alone.

We assigned individuals aged 4 to 18 years (representing 20% of the total pop-

ulation) to schools—nursery, elementary, and high school—based on their age and residential location. Each school was associated with a unique, non-overlapping catchment area within which students were assigned and grouped into age-based classes. Nursery schools covered areas of 75 by 75 households, while elementary and high schools covered areas of 50 by 60 households. When a local school exceeded its capacity (300 students), the overflow was redirected to larger central schools with a capacity of 600 students. This assignment process resulted in two types of schools: local schools, composed of students living nearby, and central schools, which bring together students from across the city.

The chosen school sizes fall within the range reported in European sociodemographic data [3, 4]. Since we are modeling a scenario with contact restrictions in place, only within-class interactions are considered. Each class consists of 25 students ($Sch_1$), a number consistent with the average reported across student types in [4]. To reflect stronger and more frequent interactions among close peers, each class is further subdivided into smaller friendship-based groups ($Sch_2$) of 8 to 9 students.

Individuals aged 20 to 65 years (60% of the total population) were assigned to work-related activities ($W$). We only consider interactions within workgroups, assuming that interactions between different groups within workplaces were inhibited due to the restrictions in place. Workgroup sizes were sampled from a Poisson distribution with a mean of 6. Although detailed data on workplace sizes are limited and context-dependent, available statistics from Italy and the United Kingdom show broadly similar patterns [3]. Notably, the proportion of groups with 5 to 9 members—nearly half of all workplaces—closely matches empirical observations, suggesting that our simple approach yields realistic group structures. Deviations in other size ranges are to be expected, as the restrictions in place naturally limit the formation of larger contact groups.

To account for interactions arising from encounters in locations such as gyms, pharmacies, and retail stores or boutiques ($B$), the city includes 900 $B$-places, each of which can be frequented by up to 300 different agents who may interact there. Assignments are made based on spatial proximity: random coordinates are selected for each location, which is then associated with a square area of influence measur-

ing 90 units per side on the grid. These squares may overlap with those of other $B$-places. The 300 agents assigned to each $B$-place are randomly selected from residents over the age of 12 living in households within the corresponding square. This approach introduces heterogeneity, as some individuals become linked to multiple locations, while others may not be linked to any. These places represent a set of routine destinations that individuals might frequent. Importantly, we chose not to include workers associated with these locations—such as store employees—in these interactions. This exclusion is justified under the assumption that high-contact occupations may adopt stricter protective measures, effectively offsetting the potential hub-like effect of their elevated exposure.

After assigning all the types of contacts already described ($Q$, $H$, $Sch_1$, $Sch_2$, $W$, and $B$), we observed that some households were only connected through the city's broader regions ($Q$). This occurs particularly for households inhabited by older, retired individuals who are not assigned to any workplace and do not frequent any store either. To address this limited connectivity, we introduced extended family interactions beyond cohabitation. While this type of interaction may also involve less isolated households, it is especially justified for older individuals who do not visit stores, as they still need to obtain basic supplies. One plausible mechanism for this is through contact with more active family members. We therefore added an additional layer of connections linking households inhabited by individuals aged 51–75 with two other households inhabited by members of the 20–50 age group. These interactions do not correspond to specific physical locations, unlike the other defined *places*. The extended family ($F$) of the individuals living in house $H_i$ consists of the individuals residing in houses $H_j$ and $H_k$ (see Fig. S1). Note that house $H_j$ is not necessarily connected to $H_k$.

Finally, we wish to note that the design of this contact structure was conceived with the aim of progressively incorporating greater complexity, allowing us to tackle other problems in future studies.

## S2. Transmission Rates in Type-$B$ Locations

In this section, we describe how we have defined the transmission rates for contacts between individuals occurring in type-$B$ locations (e.g., gyms, retail stores, boutiques, etc.). For other types of locations, any two individuals $i$ and $j$ within a given location $l$ share the same transmission rate, $\beta_l$. However, this is not the case for type-$B$ locations.

Each individual $i$, older than 12 years, is associated with a number $n_B^i$ of boutiques/stores they may visit. Each day, they go to one of their $n_B^i$ assigned stores—say, store $l$—and may come into contact with individual $j$, who is also a visitor of that store. The probability rate of infecting individual $j$, $r_l^j$, is taken to be inversely proportional to the number of stores $j$ visits, $n_B^j$, since the greater the value of $n_B^j$, the less likely it is that individual $j$ is present in location $l$ on that day:

$$r_l^j = \frac{\beta_B}{n_B^j S_l}, \text{ with } S_l = \sum_{k\in l} \frac{1}{n_B^k} \tag{1}$$

Then, the transmission rate between individuals $i$ and $j$ at a shared location $l$ is given by:

$$\beta_l^{(ij)} = \frac{\beta_B}{n_B^i n_B^j S_l}, \text{ with } S_l = \sum_{k\in l} \frac{1}{n_B^k} \tag{2}$$

With this definition, $\beta_l^{(ij)} = \beta_l^{(ji)}$, as expected, and all individuals have approximately the same number of contacts per unit time in $B$-type locations. In fact, the total transmission rate of individual $i$ at $B$-type locations is given by:

$$\sum_l \sum_{j\neq i} \beta_l^{(ij)} = \frac{\beta_B}{n_B^i} \sum_l \frac{1}{S_l} \sum_{j\neq i} \frac{1}{n_B^j} \sim \beta_B \tag{3}$$

since $l$ runs over their $n_B^i$ assigned locations, and the sum $\sum_{j\neq i} 1/n_B^j \sim S_l$, as it differs from $S_l$ in only one term.

Note that in the particular case where all individuals frequent only one $B$-type location, i.e., $n_B^i = 1$ for all $i$, we have $S_l = 1/N_l$ and $\beta_l^{(ij)} = \beta_B/N_l$ for all $i, j$. In this case, Eq. (3) in the main text also applies to $B$-type locations.

## S3. Simulation Algorithm

To simulate the model described in section 2.1.1 (main text) we may proceed as follows:

1) At a given day, we go through each infected individual, $i$, in the system and enter each of their assigned locations.

2) At each location, $l$, we go through every susceptible individual in the location and infected it with probabilty $p_l = 1 - e^{-\beta_l \Delta t}$.

For the locations H and F we proceed exactly like this. For the other locations, however, this procedure would be too time consuming. For the location Q, for example, $S^{(Q)}$ random numbers should be needed for each infected individual in order to perform step 2) (being $S^{(Q)}$ the number of susceptible individuals at location $Q$). The number of infections produced by the infected individual, $i$, would be given by a binomial distribution with mean:

$$k_i = S^{(Q)}(1 - e^{-\beta_l \Delta t}) = S^{(Q)}(1 - e^{-\frac{\beta_T}{N_l}\Delta t}) \sim \frac{S^{(Q)}}{N_l}\beta_T \Delta t \tag{4}$$

since $\beta_T \Delta t / N_l \ll 1$. On the other hand, the probability of obtaining more than one infected individual is extremely low. Then, in this case, instead of step 2) we perform step:

2') At each location, $l$, we choice an individual randomly and, if susceptible, we infected it with probability $p = 1 - e^{-\beta_T \Delta t}$

In this case, only 0 or 1 individuals could result infected at each time-step, at each location, from the infected individual, $i$. The mean number of infections produced by infected $i$ is given by the product of the probability of choosing a susceptible individual among the $N_l$ and the probability of infect it that, for location $Q$, is:

$$k_i = \frac{S^{(Q)}}{N_l}(1 - e^{-\beta_T \Delta t}) \sim \frac{S^{(Q)}}{N_l}\beta_T \Delta t \tag{5}$$

for $\beta_T \Delta t$ small enough. For $T = Q$ this condition is clarly satisfied and step 2') produce the same results as step 2) with high accuracy. However, for $T = W$, for

example, $\beta_T = 0.136$ for scenario L and the difference between performing step 2) and 2') can lead to a difference in $k_i$ of at most 6%. This difference has no impact on the analysis of the results presented, since the same algorithm was used across all scenarios—both for the determination of $R_0$ and the parameters $\beta_T$, as well as for all the simulations carried out in this work. The only consequence of using algorithm 2') instead of 2) is that the rates we use in practice are not exactly those in Table 2 (main text), but are slightly modified. Since the modification may vary slightly at work for different values of $N_l$ the dependence of $\beta_l$ on $N_l$ at work is also, in practice, slightly altered with respect to expression (3). In fact, we could have defined the model used in this work directly from the algorithm itself, but we chose the presentation in Section 2.1.1 because, although approximate, it provides a clear picture of the structure of the problem.

In summary, we use the algorithm defined by steps 1) and 2) for $T = H, F$, and by steps 1) and 2') for $T \neq H, F$.

*Doubling the rates.*

For the particular case in which the rates are multiplied by 2, instead of multiplying the $\beta_T$ by 2, we perform step 2') by selecting randomly 2 individuals instead of 1 (in the case where $N_l$ =1, the same individual is selected twice). A careful analysis of the probabilities involved in this case shows that the relative differences compared to what would be obtained using steps 1) and 2) are even smaller than those mentioned before, for $\beta_T = 0.136$.

## S4. Fraction of contacts occurring in each type of location.

This section presents the computation of the fraction of contacts, $f_T^C$, occurring in each type of location $T$, with the purpose of comparing them with findings reported in the literature.

$$f_T^C = \langle n_T \rangle / \langle n \rangle, \text{with } \langle n \rangle = \sum_T \langle n_T \rangle \quad (6)$$

where $\langle n_T \rangle$ is the average number of daily contacts per individual occurring in locations of type $T$. Since we have assumed a transmission probability per contact of the same magnitude for all contacts ($\beta_l = c_t \beta_l^C$), computing the fraction of daily

contacts occurring in a given location is equivalent to computing the fraction of infective contacts, and will be independent of the value of $c_t$. Therefore, in what follows, we set $c_t = 1$. A contact between individuals at location $l$ is modeled as a Poisson process with rate $\beta_l$; thus, through each link, each individual has an average of $\beta_l$ daily contacts. We now compute the average number of daily contacts in each type of location.

*Home (H)*

All individuals living in households of 2 or 4 people have home contacts. The average number of home contacts is given by: $\langle n_H \rangle = \beta_H (1.f_H^1 + 3.f_H^3)$ where $f_H^k$ is the fraction of $k$-individual households, and the result is approximately 1.82 $\beta_H$.

*Family (F)* To estimate the average number of daily contacts per individual in location $F$, we compute the total number of contacts occurring in location $F$, $N_F^C$, and then divide it by the total number of individuals. This gives approximately: $\langle n_F \rangle = 1.7\beta_F$.

To compute $N_F^C$, we count the family contacts of individuals living in 4-person households: $\beta_F \cdot 4 \cdot (2n_{11} + 3n_{12} + 4n_{22}) = N_F^C/2$ where $n_{ab}$ is the number of 4-person households connected to families composed of $a$ and $b$ individuals. The total number of contacts $N_F^C$ is twice this amount, since the remaining families involved in extended-family interactions live in 1- and 2-person households, all of which are connected to 4-person households.

*Work (W)*

60% of the individuals have contacts at work, and all have the same average number of daily contacts $\beta_W$, so $\langle n_W \rangle = 0.6\beta_W$.

*School ($S_1$ and $S_2$)*

20% of the individuals have contacts at school, and all have the same average number of daily contacts at locations $S_1$ and $S_2$, so the average number of daily contacts at school is $\langle n_S \rangle = 0.2(\beta_{S_1} + \beta_{S_2})$.

*Stores and Boutiques (B)*

Only individuals older than 12 years go to stores and have an average of $\beta_B$ daily contacts there. Therefore, the average number of daily $B$-type contacts computed over the whole population is $\langle n_B \rangle \sim (63/75)\beta_B \sim 0.84\beta_B$.

*Quarter (Q)*

All individuals have $\beta_Q$ average daily contacts in their quarter, so $\langle n_Q \rangle = \beta_Q$.

### S5. Mean time an individual is infectious, $\langle \tau_{inf} \rangle$

Here, we calculate the average time an individual remains infectious, assuming an exponential distribution of recovery times and considering an algorithm where the state of individuals is updated at each discrete time interval $\Delta t$. We then divide the time axis into a sequence of times $t_i = i\Delta t$, $i = 0, 1, 2, ...$ which define intervals $\Delta_i \equiv (t_{i-1}, t_i)$, $i = 1, 2, ...$, all of length $\Delta t$. Starting from the fact that the probability of an individual recovering between $t$ y $t + dt$ is $\gamma e^{-\gamma t} dt$, we calculate the probability of an individual recovering within the interval $\Delta_i$,

$$P_r(i) = \gamma \int_{i-1}^{i} e^{-\gamma t} dt = e^{-\gamma t_{i-1}} (1 - e^{-\gamma \Delta t}) \tag{7}$$

In our algorithm, the individual remains infectious throughout the interval $\Delta_i$ and transitions to the recovered state at the instant $t_i$. Therefore, the average time an individual remains infectious is given by

$$\langle t_{inf} \rangle = \sum_{i=1}^{\infty} t_i P_r(i) = \sum_{i=1}^{\infty} i \Delta t e^{-\gamma (i-1) \Delta t} (1 - e^{-\gamma \Delta t}) = \frac{\Delta t}{1 - e^{-\gamma \Delta t}} \tag{8}$$

### S6. Probability of recovering before infecting

Let us suppose that an individual $i$ is infected in one of their accessible locations, $k$. Assume that this individual is the only infected person in another of their accessible locations, $l$. We are interested in computing the probability that individual $i$ recovers before infecting anyone in location $l$; that is, the probability that the transmission chain that could occur through $i$ between locations $k$ and $l$ is interrupted. We will carry out the calculation assuming continuous time, as it is simpler. If there are $N_l$ individuals in location $l$ who can be contacted, of which $N_S$ are susceptible, the probability $P_{rec}$ that $i$ recovers before infecting anyone in location $l$ depends on the type of recovery:

*Deterministic Recovery* (DR)

Since in this case all individuals recover after a time $\tau_{inf} = 1/\gamma$, $P_{rec}$ is equal to the probability that no infection occurs during that time interval, which is given by:

$$P_{rec} = \left[e^{-\beta_l/\gamma}\right]^{N_S} = e^{-\beta_l N_S/\gamma} \tag{9}$$

where $e^{-\beta_l/\gamma}$ is the probability that no transmission occurs during $\tau_{inf}$ through one of the $N_S$ links with susceptible individuals.

*Exponential Recovery* (ER)

In this case, there is a probability that recovery occurs at any point in time, so we need to evaluate the probability that the individual recovers before infecting. This probability can be computed as:

$$P_{rec} = a_{\text{rec}}/a_0, \text{ with } a_0 = a_{\text{rec}} + a_{\text{inf}} = \frac{1}{1 + N_S\beta_l/\gamma} \tag{10}$$

where $a_{\text{rec}} = \gamma$ and $a_{\text{inf}} = N_S\beta_l$ are the probability rates at which recovery or infection events occur, respectively, in location $l$ [5].

In summary:

$$P_{rec} = \begin{cases} e^{-\beta_l N_S/\gamma} & \text{for DR} \\ \frac{1}{1+N_S\beta_l/\gamma} & \text{for ER} \end{cases} \tag{11}$$

In Figure S4, these probabilities are plotted for both types of recovery as a function of $x = N_S\beta_l/\gamma$, with the corresponding values of $P_{rec}$ highlighted for a household of 4 individuals (circles) and a workplace (triangles), where the other $N_l$ individuals sharing the location with the infected one are susceptible.

## References


[1] J. Zhang, M. Litvinova, Y. Liang, Y. Wang, W. Wang, S. Zhao, Q. Wu, S. Merler, C. Viboud, A. Vespignani, M. Ajelli, H. Yu, Changes in contact patterns shape the dynamics of the covid-19 outbreak in china, Science 368 (2020) eabb8001. doi:10.1126/science.abb8001.

[2] M. P. V. A. M. S. Fumanelli L, Ajelli M, Inferring the structure of social contacts from demographic data in the analysis of infectious diseases spread., PLoS Comput Biol. (09 2012). doi:10.1371/journal.pcbi.1002673.

[3] S. Merler, M. Ajelli, Human mobility and population heterogeneity in the spread of an epidemic, Procedia Computer Science 414 (2010) 2237–2244. doi:10.1016/j.procs.2010.04.250.

[4] M. Ajelli, G. Jurman, C. Furlanello, C. Rizzo, A. Bella, M. Massari, C. Ciofi degli Atti, Modeling influenza pandemic in italy: An individual-based approach (01 2007).

[5] D. T. Gillespie, A general method for numerically simulating the stochastic time evolution of coupled chemical reactions, Journal of computational physics 22 (4) (1976) 403–434.

Table S1: **Transmission Parameters for scenarios with different proportions of frequent contacts.** Values of $\beta_T$ for the different location types, $T$, and various proportions, $p$, of infections occurring through frequent contacts, for both exponential (ER) and deterministic (DR) recovery settings. The scenarios corresponding to the cases with $p = 60$ and $p = 90$ are those referred to as G and L, respectively.

| | $\beta_T$ (ER) | | | | | | | |
|---|---|---|---|---|---|---|---|---|
| $T \setminus p(\%)$ | 15 | 30 | 45 | 60 (G) | 75 | 90 (L) | 95 | 100 |
| $H$ | 0.008 | 0.017 | 0.029 | 0.045 | 0.066 | 0.102 | 0.118 | 0.126 |
| $F$ | 0.001 | 0.003 | 0.005 | 0.008 | 0.012 | 0.018 | 0.020 | 0.022 |
| $W$ | 0.010 | 0.020 | 0.035 | 0.054 | 0.080 | 0.124 | 0.144 | 0.154 |
| $B$ | 0.037 | 0.030 | 0.022 | 0.018 | 0.009 | 0.004 | 0.002 | 0.000 |
| $Q$ | 0.101 | 0.083 | 0.059 | 0.047 | 0.024 | 0.012 | 0.006 | 0.000 |

| | $\beta_T$ (DR) | | | | | | | |
|---|---|---|---|---|---|---|---|---|
| $T \setminus p(\%)$ | 15 | 30 | 45 | 60 (G) | 75 | 90 (L) | 95 | 100 |
| $H$ | 0.008 | 0.018 | 0.029 | 0.042 | 0.063 | 0.098 | 0.114 | 0.151 |
| $F$ | 0.002 | 0.003 | 0.005 | 0.007 | 0.011 | 0.017 | 0.020 | 0.026 |
| $W$ | 0.010 | 0.021 | 0.035 | 0.051 | 0.076 | 0.119 | 0.139 | 0.184 |
| $B$ | 0.038 | 0.032 | 0.025 | 0.019 | 0.012 | 0.005 | 0.003 | 0.000 |
| $Q$ | 0.106 | 0.087 | 0.068 | 0.051 | 0.033 | 0.013 | 0.008 | 0.000 |

Table S2: **Fractions of Infections Occurring at Different Location Types** Fractions of infections that occur at each location type, $T$, for scenarios with different proportions, $p$, of infections occurring through frequent contacts, for exponential (ER) and deterministic (DR) recoveries. Note that the value reported for $p$ has been rounded from the average across simulations, which is provided in row 4 of each table.

| | Infections (ER) | | | | | | | |
|---|---|---|---|---|---|---|---|---|
| $T \setminus p(\%)$ | 15 | 30 | 45 | 60 (G) | 75 | 90 (L) | 95 | 100 |
| $H$ | 9.3% | 17.8% | 26.4% | 33.3% | 39.1% | 44.0% | 45.2% | 46.3% |
| $F$ | 1.7% | 3.4% | 5.7% | 8.0% | 10.5% | 13.9% | 15.0% | 16.5% |
| $W$ | 4.0% | 8.1% | 13.2% | 18.6% | 24.5% | 32.1% | 34.2% | 37.2% |
| local/frequent | 15.0% | 29.3% | 45.3% | 59.9% | 74.1% | 90.0% | 94.4% | 100.0% |
| $B$ | 18.0% | 14.9% | 11.5% | 8.4% | 5.4% | 2.1% | 1.2% | 0.0% |
| $Q$ | 67.0% | 55.8% | 43.2% | 31.7% | 20.5% | 7.9% | 4.4% | 0.0% |
| global/occasional | 85.0% | 70.7% | 54.7% | 40.1% | 25.9% | 10.0% | 5.6% | 0.0% |

| | Infections (DR) | | | | | | | |
|---|---|---|---|---|---|---|---|---|
| $T \setminus p(\%)$ | 15 | 30 | 45 | 60 (G) | 75 | 90 (L) | 95 | 100 |
| $H$ | 9.6% | 18.9% | 28.1% | 35.5% | 42.3% | 47.1% | 47.9% | 48.3% |
| $F$ | 1.7% | 3.5% | 5.5% | 7.4% | 9.9% | 12.9% | 13.8% | 15.0% |
| $W$ | 4.0% | 8.1% | 12.7% | 17.3% | 23.2% | 30.7% | 33.1% | 36.6% |
| local/frequent | 15.3% | 30.5% | 46.3% | 60.2% | 75.4% | 90.7% | 94.8% | 100.0% |
| $B$ | 18.0% | 14.7% | 11.3% | 8.3% | 5.1% | 1.9% | 1.1% | 0.0% |
| $Q$ | 66.7% | 54.8% | 42.4% | 31.5% | 19.5% | 7.4% | 4.1% | 0.0% |
| global/occasional | 84.7% | 69.5% | 53.7% | 39.8% | 24.6% | 9.3% | 5.2% | 0.0% |

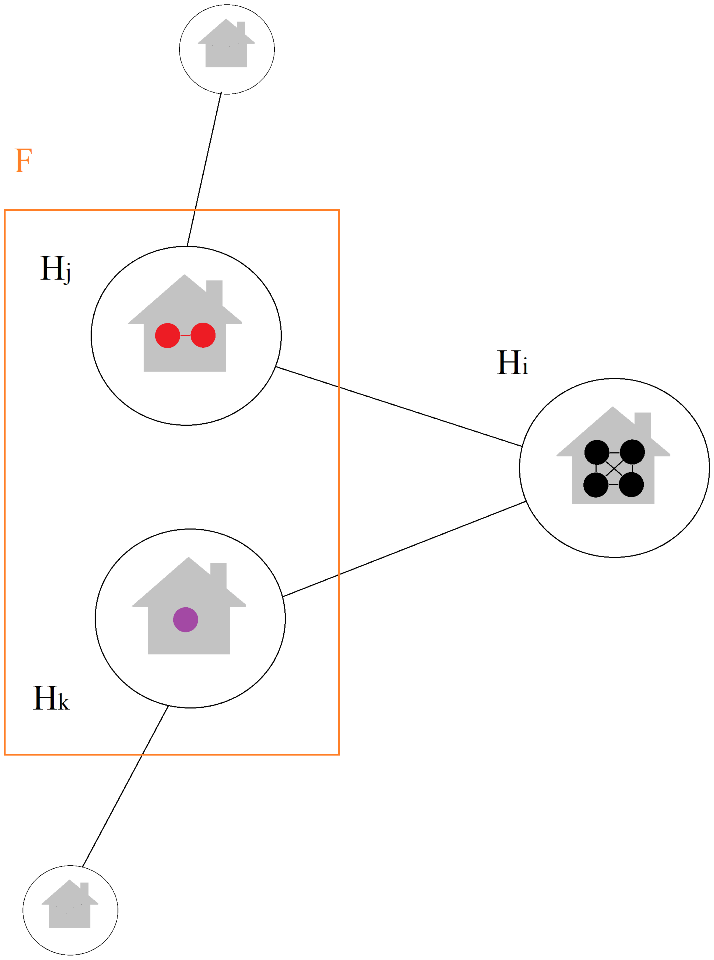


Fig. S1: **Diagram of the Extended Family Structure.** The extended Family, $F$, of individuals in house $H_i$, are all the individuals $f \in F$, where $F = H_j \cup H_k$. All the individuals in $H_i$ are connected to those in $F$, but individuals belonging to $H_j$ are not necessarily connected to those in $H_k$. The extended Family of the individuals in $H_k$ is composed of the individuals in $H_i$ and of the individuals from another household (schematized below $H_k$ in the figure).

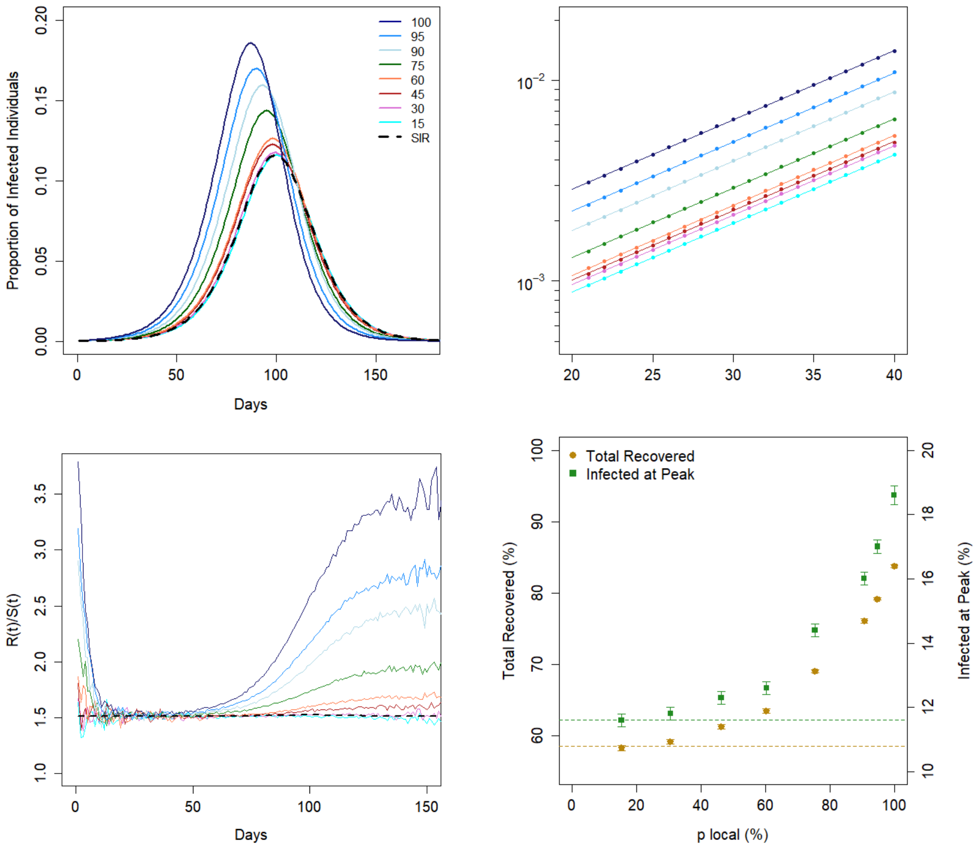


Fig. S2: **Epidemic spread in scenarios with different proportions of *local* contacts.** System dynamics for scenarios where 15% to 100% of infections are produced through frequent contacts (at locations H, F and W) for D-type recovery. The colored curves represent average over 20 simulations. Deterministic SIR in discrete time (black dashed line). (a) Fraction of infected individuals. $R_0^{100\%} = 1.51{\pm}0.03$; $R_0^{95\%} = 1.51{\pm}0.04$; $R_0^{90\%} = 1.51{\pm}0.04$; $R_0^{75\%} = 1.51{\pm}0.04$; $R_0^{60\%} = 1.51 \pm 0.04$; $R_0^{45\%} = 1.51 \pm 0.05$; $R_0^{30\%} = 1.51 \pm 0.06$; $R_0^{15\%} = 1.51 \pm 0.04$. $R_0^{SIR} = 1.51$. (b) Same as figure (a) for the start of epidemic spread. The results of the simulations (points) and an exponential fit (lines) are shown in logarithmic scale. (c) Ratio between reproductive ratio and fraction of susceptible individuals, $R(t)/s(t)$. (d) Fraction of the population infected at the peak (yellow points) and total fraction of the population infected (green points) as a function of the percentage $p$ of infections that are produced through frequent contacts.

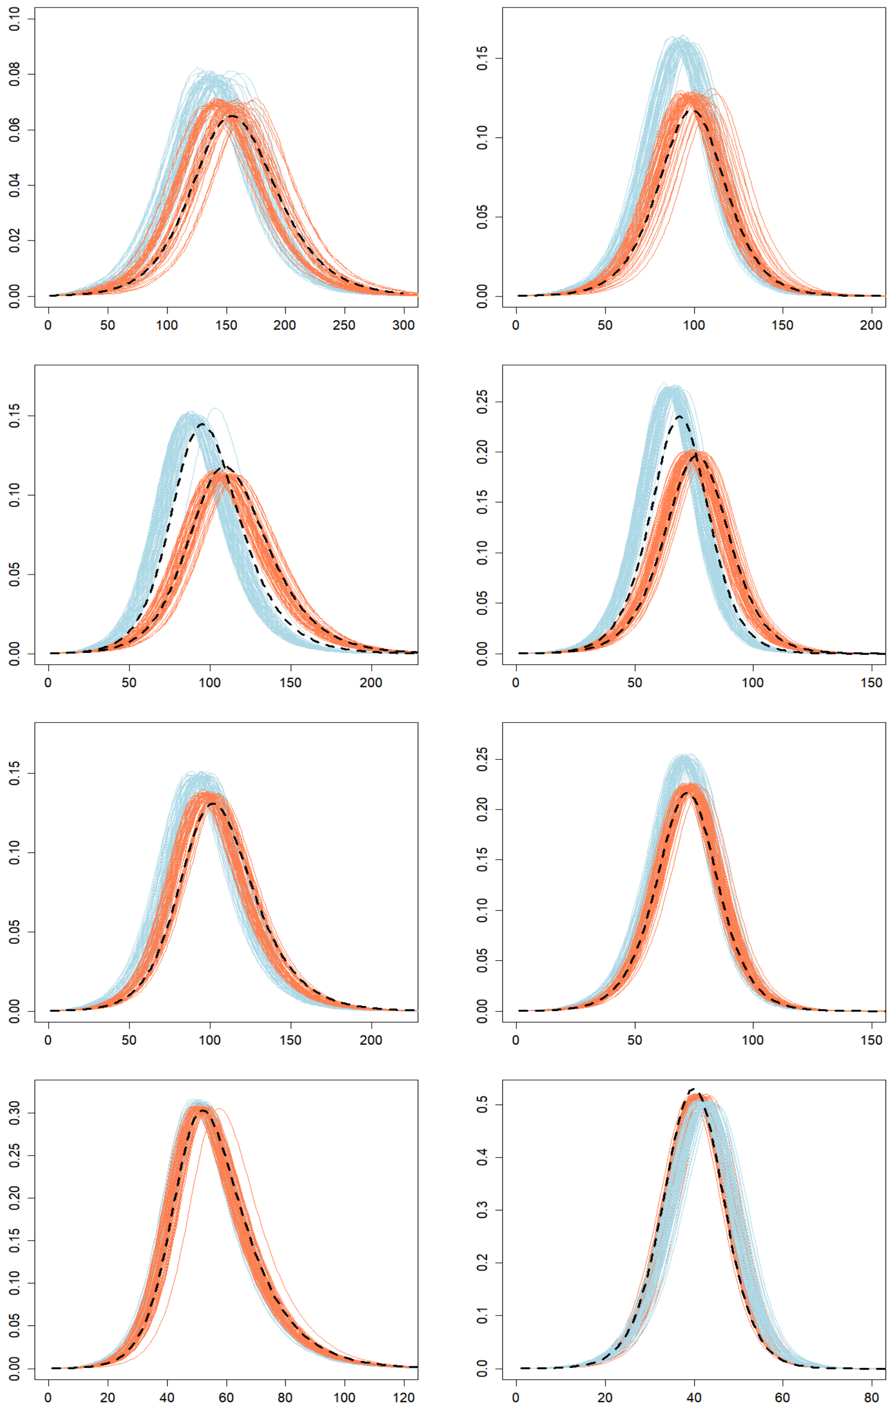


Fig. S3: **Comparison of IBM results with Homogeneous Mixing predictions.** Rows 1–4 of this figure compare the curves from the 50 simulations performed with the individual-based model (colored curves), already shown in Figures 1–4 (main text), with the corresponding HM prediction (black dashed line). In the plots in rows 1, 3, and 4, the black curve corresponds to the solution of the deterministic SIR model (see Section 2.3) with $\mathfrak{R}_0$= 1.5, $\mathfrak{R}_0$= $f \cdot 1.5$ (with $f = 1.24$ for ER and 1.2 for DR), and $\mathfrak{R}_0$=3, respectively. The values $f \cdot 1.5$ and 3 are those predicted by the HM approximation when the transmission rates of the baseline case ($\mathfrak{R}_0$=1.5) are multiplied by $f$ and 2, respectively. In the plots in the second row, the black curves correspond to the SIR model results using the effective $\mathfrak{R}_0$ obtained from the agent-based model (given in the caption of Fig. 2), since in this case there is no straightforward a priori prediction of $\mathfrak{R}_0$ from the original value of 1.5.

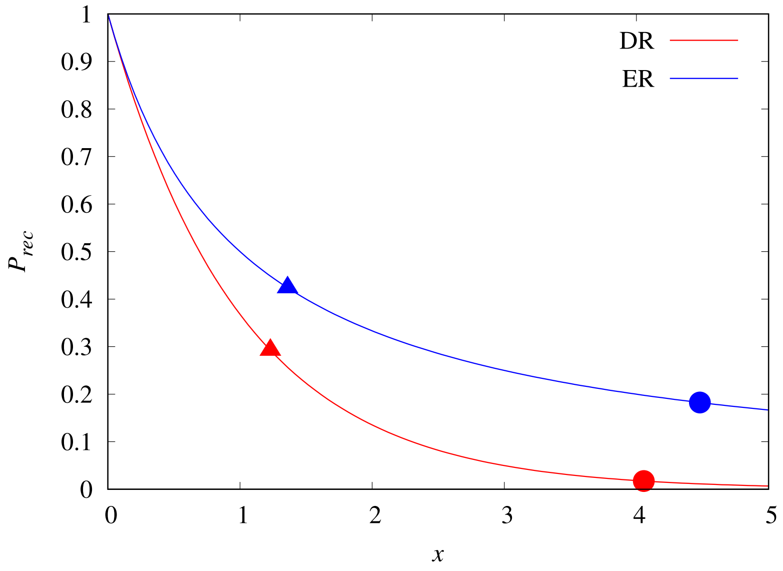


Fig. S4: **Probability of recovering before infecting for deterministic and exponential recovery.** Probability, $P_{rec}$, that an infected individual recovers before infecting anyone in a given location $l$ as a function of $x = \beta_l N_S/\gamma$ for determinisitc (DR) and exponential (ER) recovery. Here $\beta_l$ is the transmission rate per link at location $l$ given by Eq.(3) (main text), $N_S$ is the number of susceptible individuals at location $l$ and $\gamma = 1/\tau_{inf}$. The symbols indicate the values obtained when $x$ is computed for specific locations in scenario L and where $N_S = N_l$; circles: four-person households, triangles: workplaces of size $N_l + 1$ (note that $x = \beta_W/\gamma$ for all $N_l$-values).
